# Supplementary material for: FS-Net: Full Scale Network and Adaptive Threshold for Improving Extraction of Micro-Retinal Vessel Structures
Source: arXiv:2311.08059 source file (2025-01-03)
Supplement: Supplementary file 1 [file appendix.tex]

% \appendix

% \section{Sample Appendix Section}
% \label{sec:sample:appendix}
